# Supplementary material for: Local monitoring of atmospheric transparency from the NASA MERRA-2 global assimilation system
Source: arXiv:1906.01967 source file (2019-10-07)
Supplement: Supplementary file 1 [file supplement.tex]

Global temperature and moisture information is determined from the direct assimilation of satellite radiances (Cross-track infrared Sounder, Atmospheric Infrared Sounder, Infrared Atmospheric Sounding Interferometer, Microwave imager (see \citealt{mccarthy}). Assimilation of satellite radiances are performed using radiative transfer calculations 
(Community Radiative Transfer Model). It performs forward radiative transfer calculations of brightness temperature from input profiles of temperature, moisture, and ozone. A variational bias correction is applied to each channel of each instrument on each platform. It is updated at the end of each assimilation and is used as input in the subsequent analysis cycle.

\begin{figure}
\centering
\includegraphics[width=0.4\linewidth]{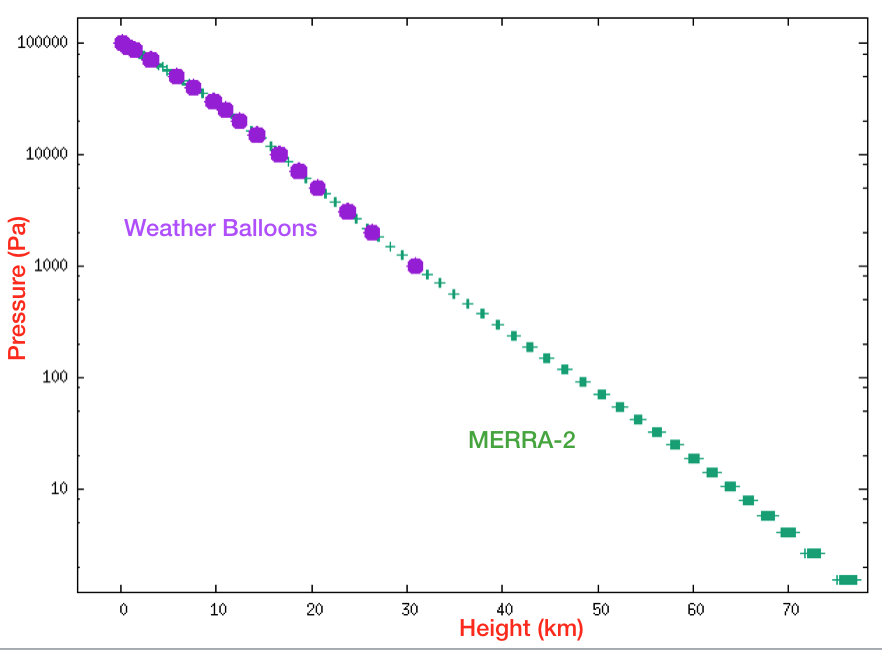}
\includegraphics[width=0.4\linewidth]{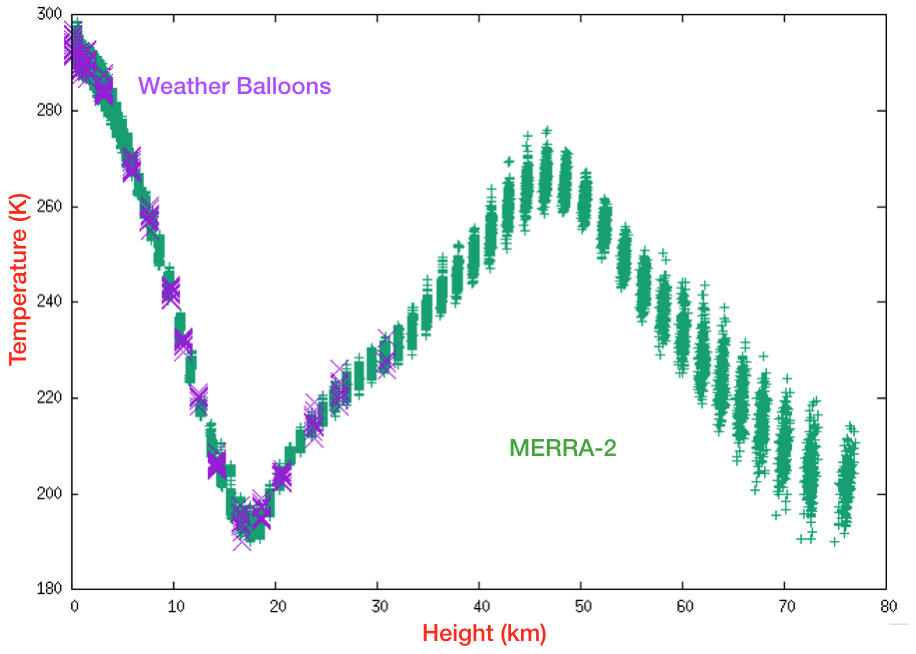}
\caption{Daily
 Barometric pressure and temperature profile Above Antofagasta. January 2017.
 \label{fig:8}}
\end{figure}

Both temperature and pressure from weather balloons and from MERRA-2 are well correlated (figure \ref{fig:8}).

 Analysis of the daily variation of air columns above Antofogasta \footnote{\url{https://confluence.lsstcorp.org/display/DM/2018-08-21+Calibration+Products+Standup}} shows that it is sufficient to input a single parameter, the local barometric pressure, to reliably inform LibRadTran molecular scattering. 

The spatio-temporal interpolation of the barometric pressure and temperature profiles has been tested against measurements from weather balloons launched from Antofogasta Airport: using either dataset impacts the molecular scattering is below the 1‰ level. 

Above Mauna Kea, Peak-to-peak variation of 6 mbar around 616 mbar. 
Dispersion of 2 mbar which translate into 2 mmag/airmass at the blue edge.
